# Supplementary material for: Learning to Track from Privileged Target Appearances
Source: arXiv:2609.02471 source file (2026-09-25)
Supplement: Supplementary file 1 [file X.appendix.tex]

\appendix
\section{Appendix}
May include other additional sections here.
